# Supplementary material for: Model-driven Cluster Resource Management for AI Workloads in Edge Clouds
Source: arXiv:2201.07312 source file (2022-01-18)
Supplement: Supplementary file 1 [file appendix_images.tex]

\begin{figure*}[t]%
\centering
\begin{minipage}[b]{0.4\linewidth}
% MP large Models
    \centering
    \includegraphics[width=\linewidth]{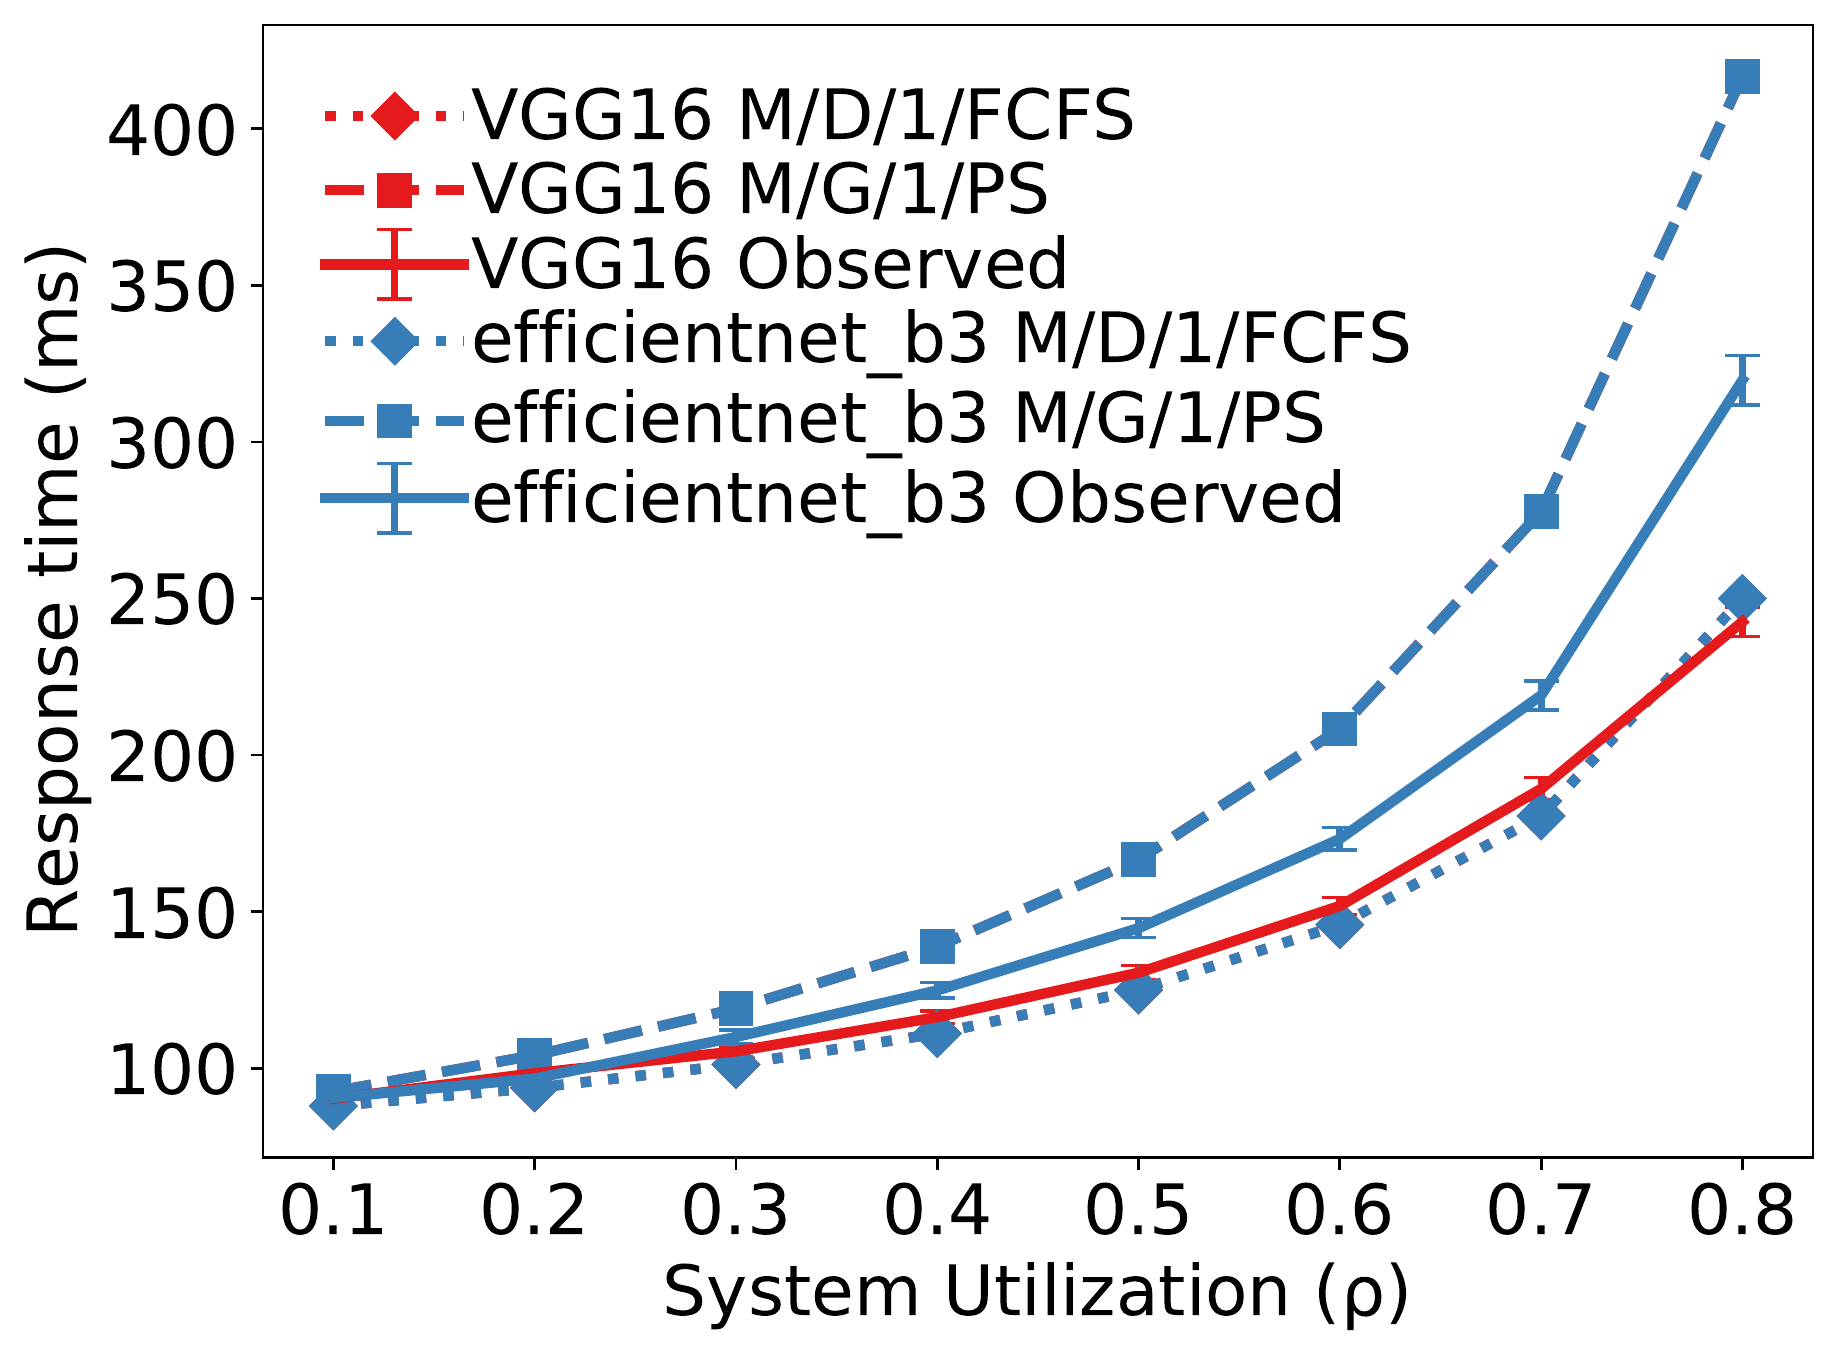} 
    \caption{GPU Validation with large models}%
\label{fig:nano_mp_large}%
\end{minipage}
\quad
\begin{minipage}[b]{0.4\linewidth}
 %MPS three models
    \centering
    \includegraphics[width=\linewidth]{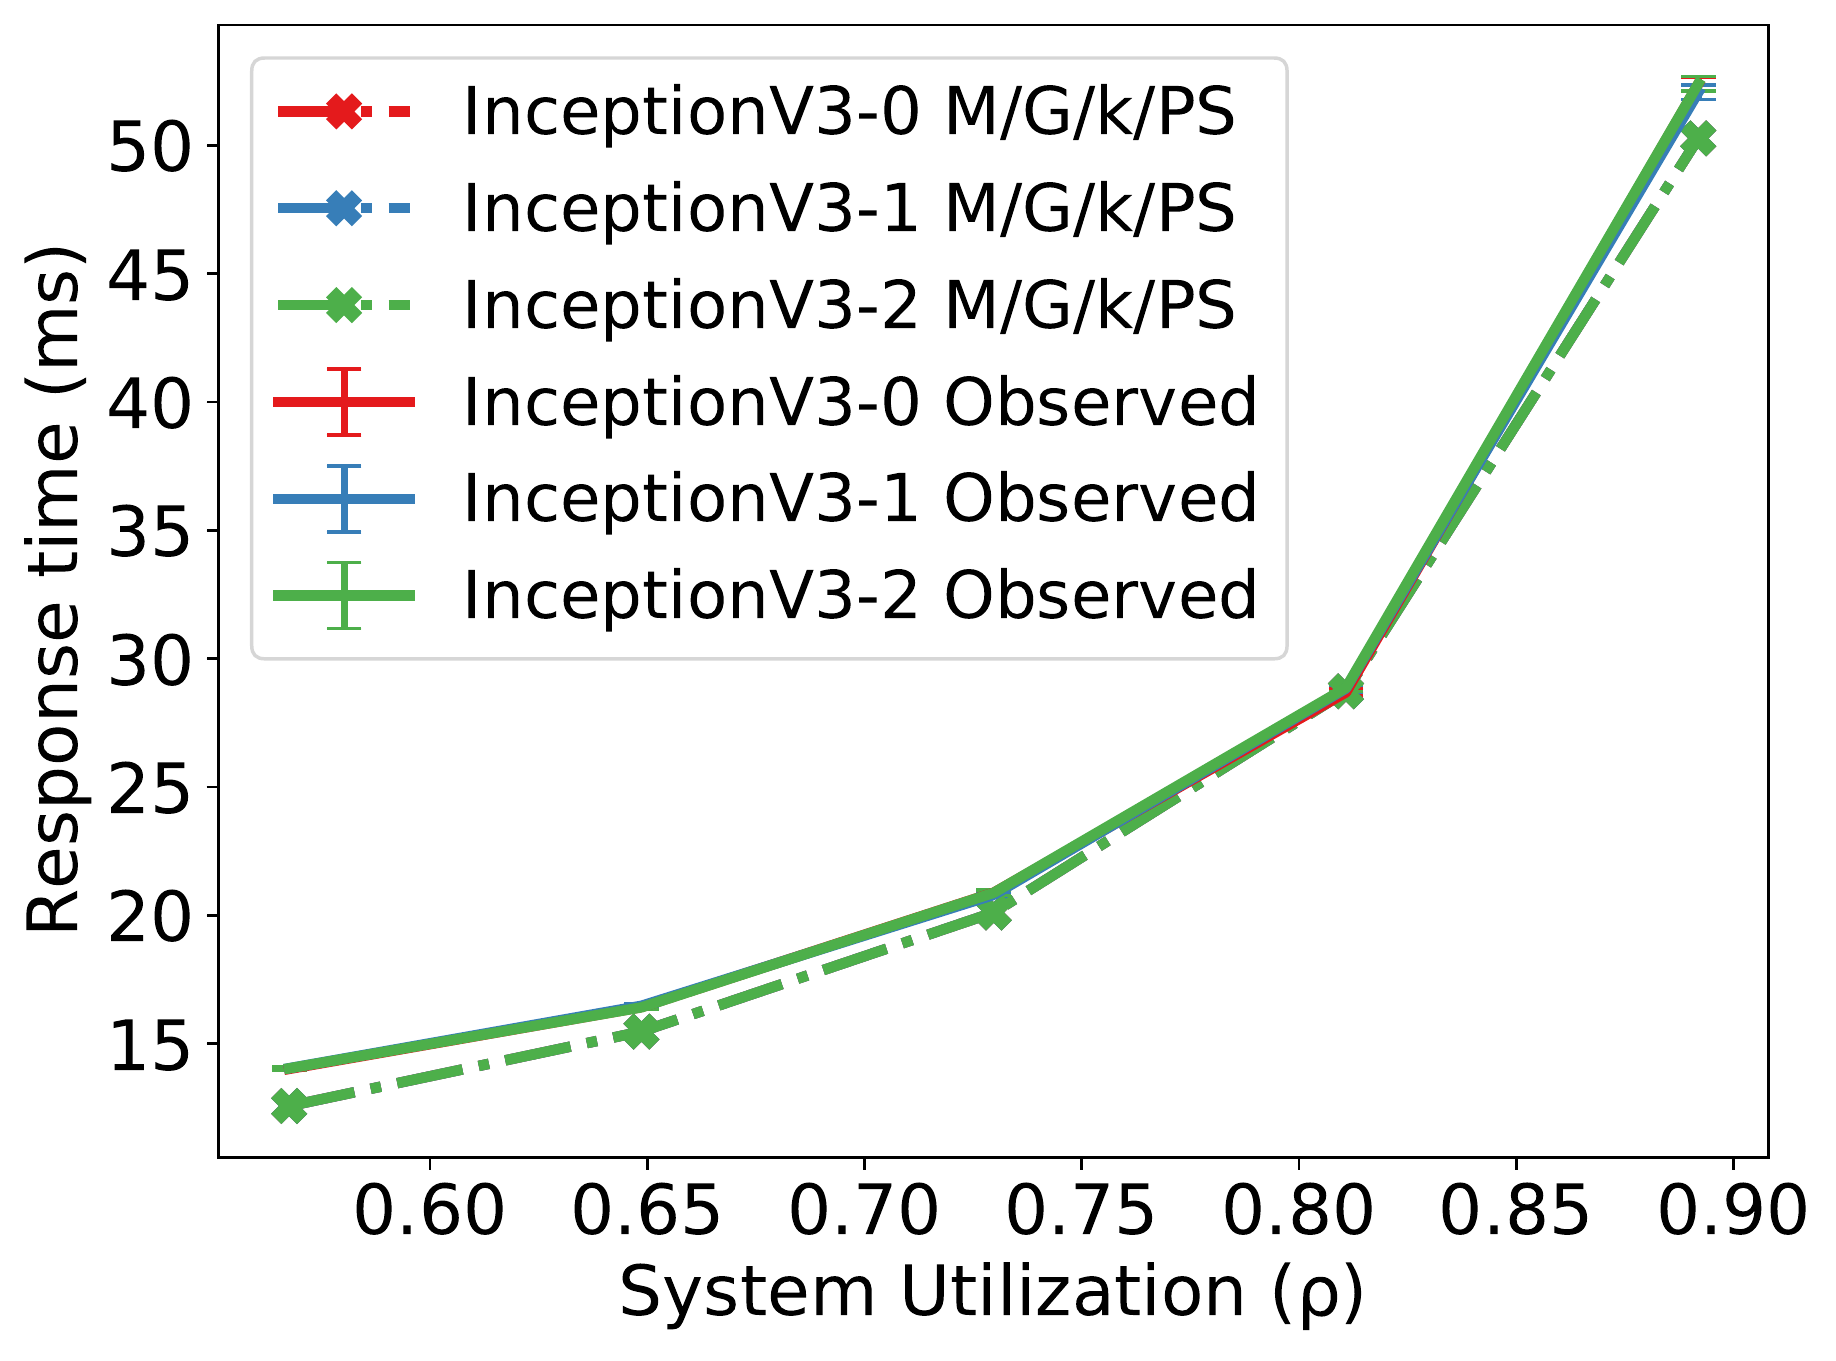} 
    \caption{MPS Validation of Three Models}%
\label{fig:mps_multiprocess_validation_3}%
\end{minipage}
\end{figure*}
