# Supplementary material for: Model-driven Cluster Resource Management for AI Workloads in Edge Clouds
Source: arXiv:2201.07312 source file (2022-01-18)
Supplement: Supplementary file 2 [file edgetpu_queuing_appendix.tex]

% EdgeTPU queuing validation
  \begin{figure*}[t]
	\centering
	\subfloat[]{
		\includegraphics[width=0.32\textwidth]{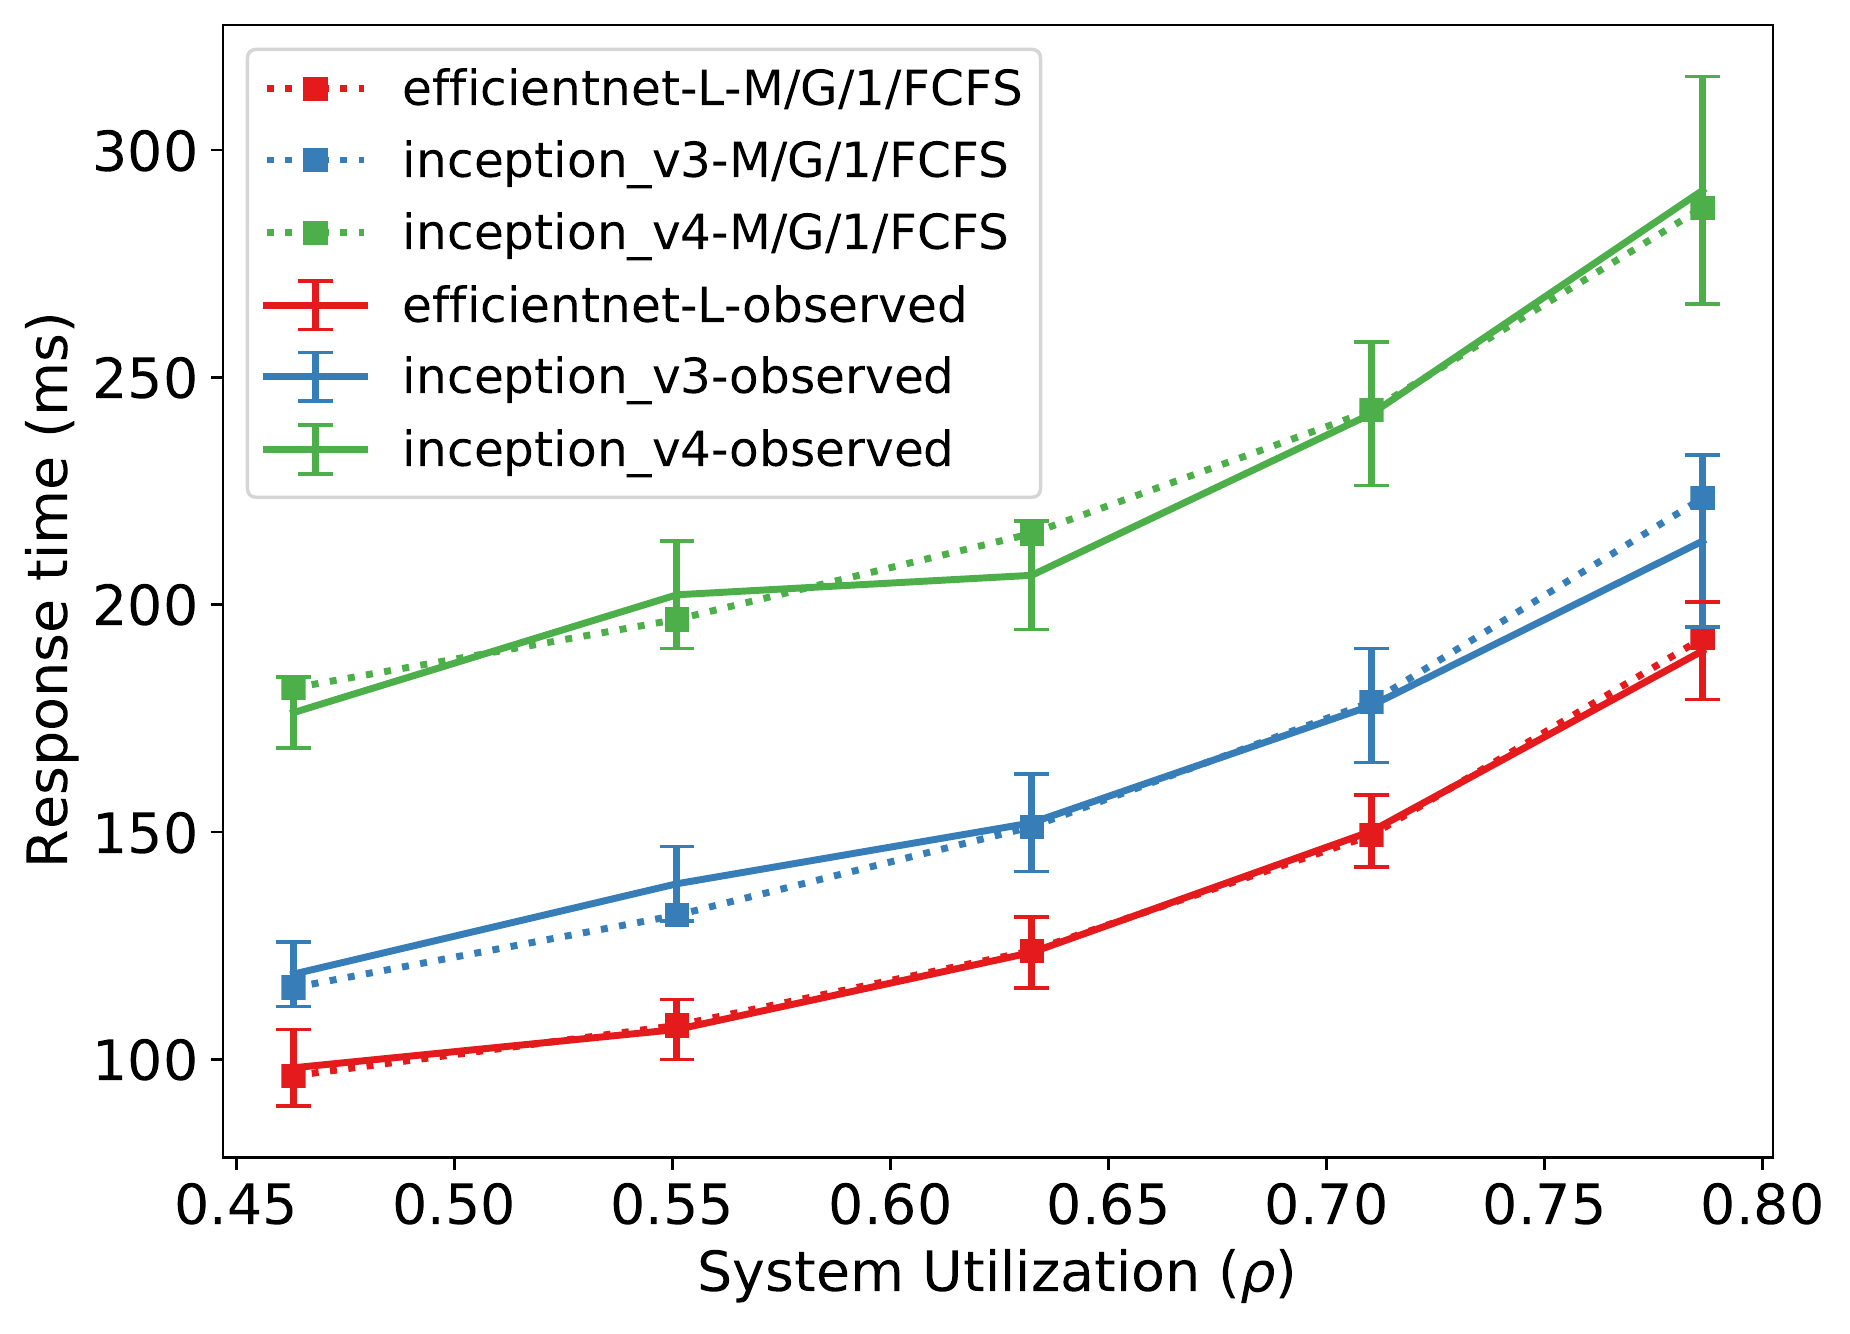}
	} 
	\subfloat[]{
		\includegraphics[width=0.32\textwidth]{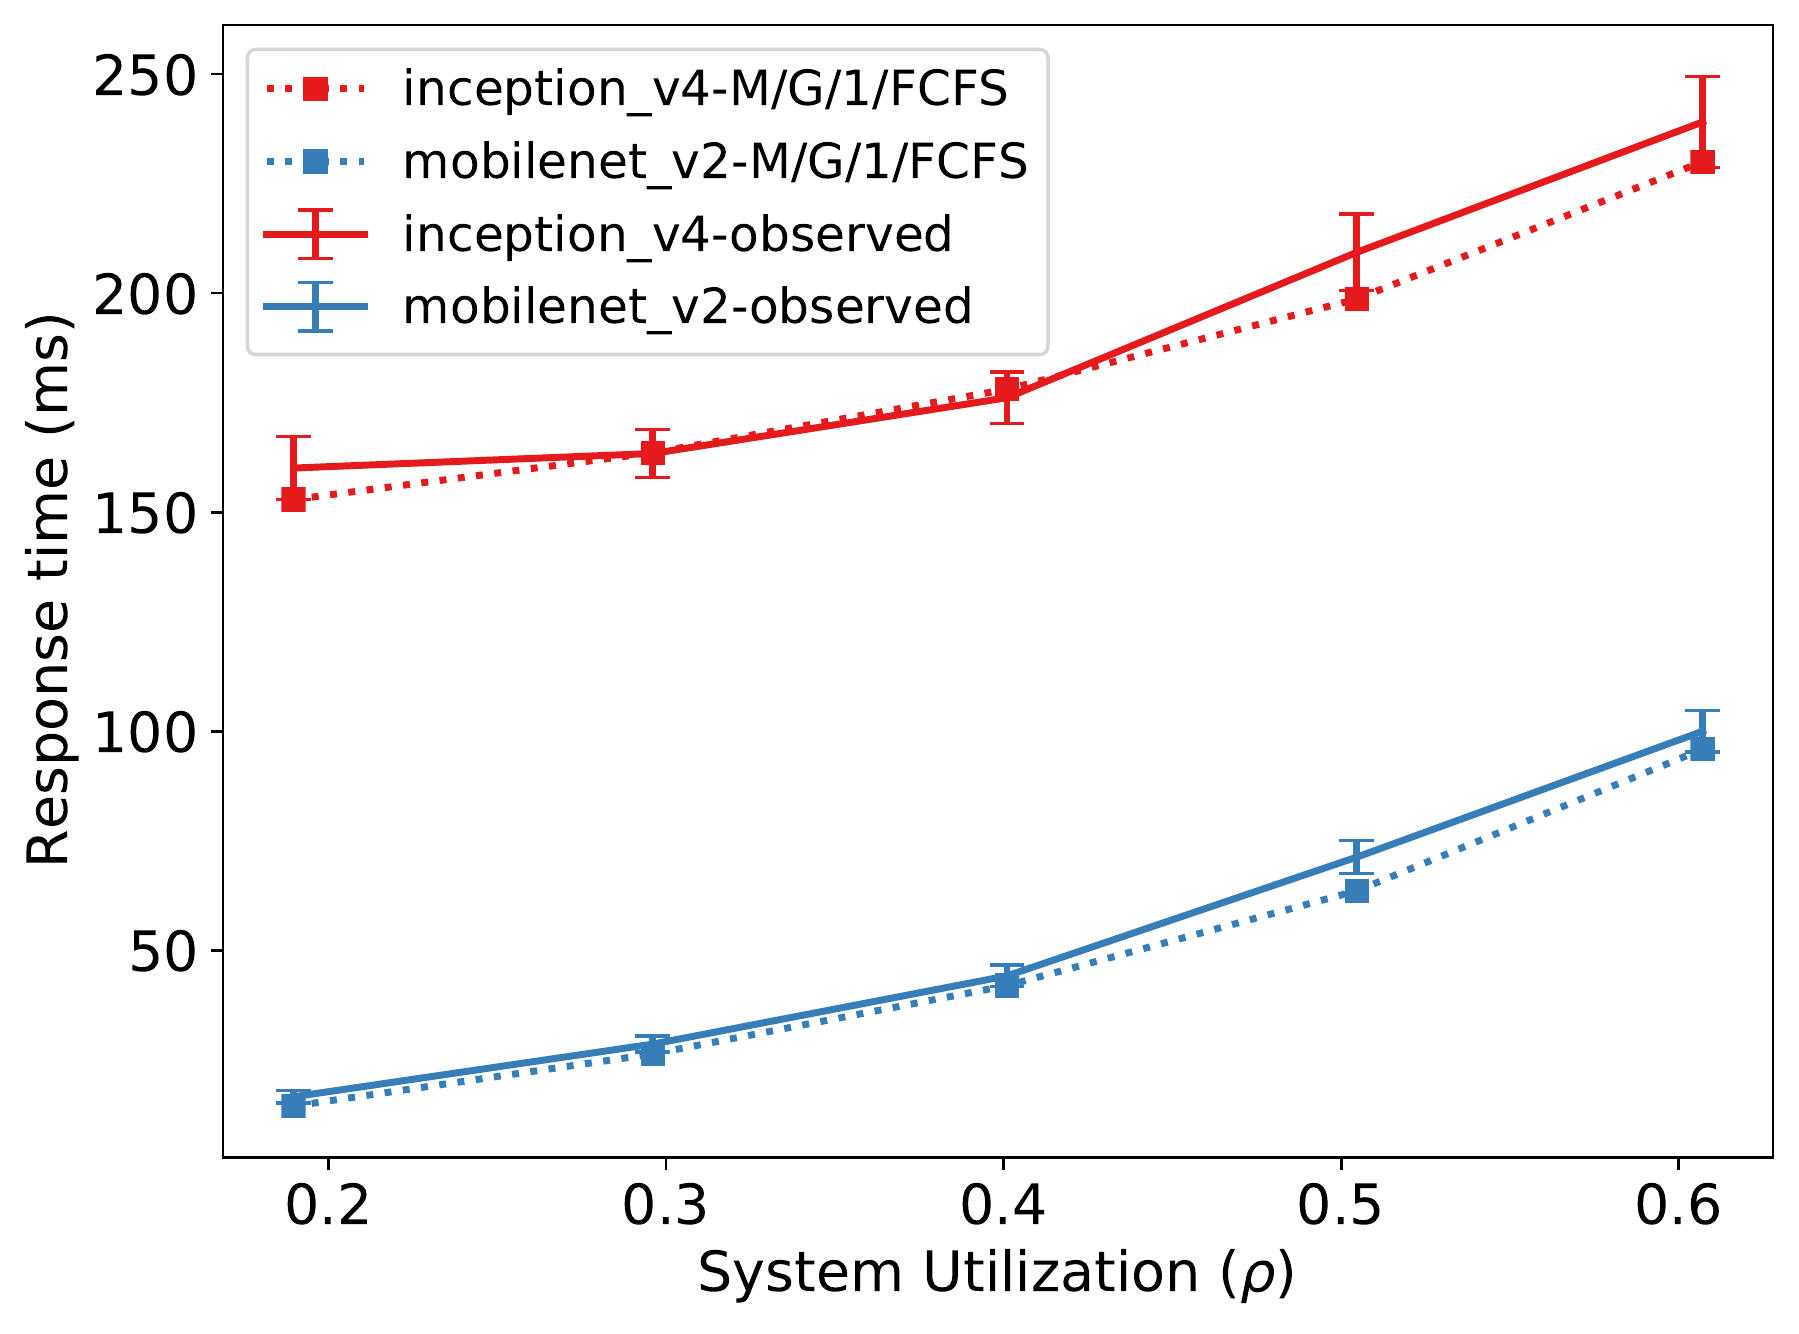}
	} 
	\subfloat[]{
		\includegraphics[width=0.32\textwidth]{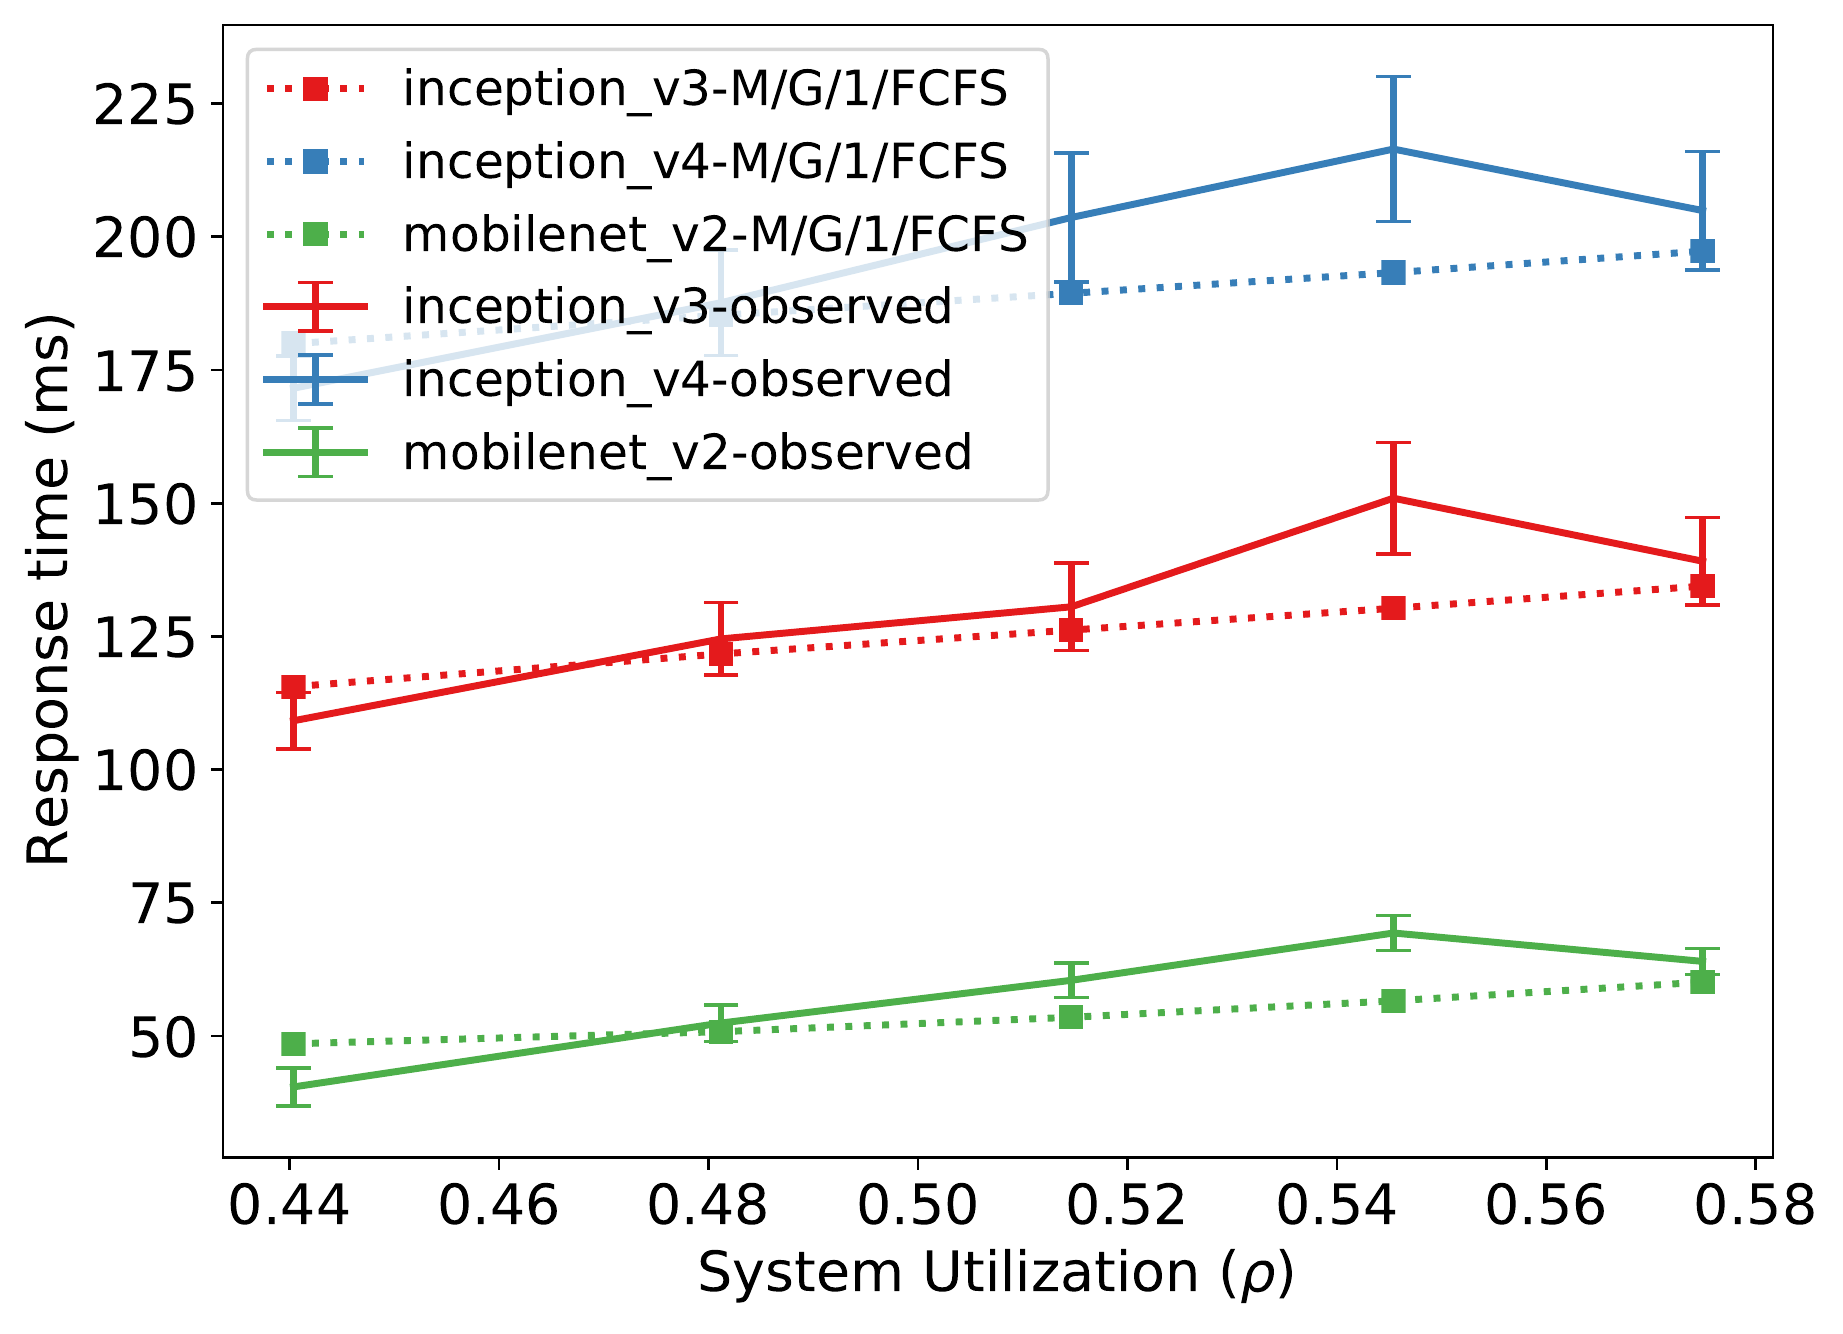}
	}
	\caption{EdgeTPU observed response time vs. M/G/1/FCFS predicted response time.}
	\label{fig:edgetpu_queue_appendix}
\end{figure*}
