# Supplementary material for: Model-driven Cluster Resource Management for AI Workloads in Edge Clouds
Source: arXiv:2201.07312 source file (2022-01-18)
Supplement: Supplementary file 3 [file appendix.tex]

\appendix
\section*{Appendices}

\section{DNN Models Characteristics}\label{apx:models}
